# Supplementary material for: Variation of Gender Biases in Visual Recognition Models Before and After Finetuning
Source: arXiv:2303.07615 source file (2023-03-14)
Supplement: Supplementary file 1 [file appendix.tex]

\subsection{COCO 2017 Analysis Set}
\begin{figure}[th]
    \centering {{\includegraphics[width=\textwidth]{figures/coco_pairs.pdf} }}%
    \label{fig:example}%
\end{figure}

\begin{figure}[th]
    \centering {{\includegraphics[width=\textwidth]{figures/coco_indiv.pdf} }}%
    \label{fig:example}%
\end{figure}

\subsection{Open Images Model Predictions}
\begin{figure}[th]
    \centering {{\includegraphics[width=\textwidth]{figures/oi_preds.pdf} }}%
    \label{fig:example}%
\end{figure}

\subsection{COCO 2017}

\subsubsection{CLIP ViT/32-B}

\subsubsection{ResNet50}

\subsubsection{ResNet18}

\subsubsection{Big Transfer ResNet50}

\subsubsection{MoCo ResNet50}

\subsubsection{SimCLR ResNet50}

\subsection{Open Images} 

\subsubsection{CLIP ViT/32-B}

\subsubsection{ResNet50}

\subsubsection{ResNet18}

\subsubsection{Big Transfer ResNet50}

\subsubsection{MoCo ResNet50}

\subsubsection{SimCLR ResNet50}
